# Supplementary material for: Using Causal Analysis to Learn Specifications from Task Demonstrations
Source: arXiv:1903.01267 source file (2019-03-04)
Supplement: Supplementary file 1 [file appendix.tex]

\section*{Appendix}
The following Figures.\ref{fig:careful_BIG}, \ref{fig:normal_BIG}, \ref{fig:aggressive_BIG} illustrate multiple cases, where the trajectory was augmented based on backpropagating through the specification model.

\begin{figure*}[]
\centering
\includegraphics[width=.95\linewidth]{images/backprop/careful/careful_BIG}
\caption{Perturbed trajectories to fit a careful user specification.}
\label{fig:careful_BIG}
\end{figure*}

\begin{figure*}[]
\centering
\includegraphics[width=.95\linewidth]{images/backprop/normal/normal_BIG}
\caption{Perturbed trajectories to fit a normal user specification.}
\label{fig:normal_BIG}
\end{figure*}

\begin{figure*}[]
\centering
\includegraphics[width=.95\linewidth]{images/backprop/aggressive/aggressive_BIG}
\caption{Perturbed trajectories to fit an aggressive user specification.}
\label{fig:aggressive_BIG}
\end{figure*}
